# Supplementary material for: The Emperor's New Autofill Framework: A Security Analysis of Autofill on iOS and Android
Source: arXiv:2104.10017 source file (2021-09-28)
Supplement: Supplementary file 2 [file appendix-history.tex]

%!TEX root = main.tex

\section{Evolution of Mobile Autofill}\label{appx:evolution}
In this section, we describe the evolution of autofill frameworks on iOS and Android.
In our work, we evaluated the iOS app extensions and Password AutoFill frameworks as well as the Android autofill service.

\subsection{Autofill on iOS}
There are five ways autofill is handled in iOS: copy and paste, in-app browsers, autofill in browsers using browser-based password managers, using app extensions (introduced in iOS 8) [2014], and using the iOS Password Autofill framework (introduced in iOS 12 [2018]).

\subsubsection{Copy and Paste}
Prior to iOS 8, non-browser based password managers required the user to first open the password manager, select the appropriate credential, copy the username and password (separately), switch to the target app, and finally paste their credentials.
Not only is this a poor usability experience, but this leaves users credentials at risk because other apps can also access the credentials stored in the clipboard.
While iOS limits clipboard access to foreground apps, there is still the possibility that a malicious app opened in the future could access a previously copied password.
This can be made even more likely by having the malicious app be a widget displayed on the users ``Today'' screen~\cite{mysk2020clipboard}.

\subsubsection{In-App Browser}
One early approach taken by mobile passwords managers was to implement a fully functional browser as part of the password manager app.
While this approach provides the most accurate autofill experience, it is less than unusable in that it does not help users authenticate to the numerous other applications on the mobile device.
While some password managers continue to provide this functionality, it is not the preferred method for autofill anymore.

\subsubsection{Browser-Based Password Manager}
Many browsers on iOS provide their own password manager, which can then be used to autofill passwords into websites displayed through the browser.
While this does work even if app extensions or Password AutoFill are unavailable, this approach is limited in that it cannot be used to autofill credentials into other apps.

\subsubsection{App Extensions}

App extensions allow a host app to interact with another app (e.g., a password manager) using a predefined set of extension features.
This approach requires both the password manager to implement the set of functions associated with the password management extension feature and for host apps to be updated to query this extension feature.
Using app extensions is more secure and usable than the copy and paste approach, though it does have two important limitations.
First, host apps are free to request passwords for any domain and it is up to the user to ensure that only correct credentials are selected.
Second, app extensions require the modification of individual host apps, an approach that does not scale well.
Figure~\ref{fig:appextensionsui} shows the interface for app extensions, first requiring the user to select which app extension to use (see Figure~\ref{fig:selectextension}) and the selecting the credentials (see Figure~\ref{fig:selectcredential}).

While Password AutoFill is intended to replace using app extensions for password management, we note that the password management extension feature is still supported in iOS and remains functional in some password managers (e.g., 1Password, Keeper, LastPass) and host apps (e.g., Safari, Edge).
Additionally, for older devices that cannot be updated to iOS 12, app extensions remain the preferred method for password autofill.

\subsubsection{Password AutoFill}\label{sec:background:autofill}

The Password AutoFill framework provides two major benefits compared to app extensions.
First, it automatically identifies login forms in apps and websites.
It is preferred that apps add appropriate \texttt{textContentType} attributes to form fields to ensure correct login form detection, but detection will still proceed using a heuristic-based approach if these attributes are not present.
Second, Password AutoFill allows for a secure mapping between an app and the domains that should have their credentials entered into that app.
That is done by having app developers include an Associated Domains Entitlement that indicates which domains are associated with the app; the domain operator is also required to include an \texttt{apple-app-site-association} file on their website indicating which apps are allowed to use credentials for that domain.
%Figure~\ref{fig:autofillui} shows the interface for Password AutoFill, both when an associated domain can be found (see Figure~\ref{fig:rec}) and when not (see Figure~\ref{fig:norec}).

\subsection{Autofill on Android}

While the evolution of autofill on Android is similar to that of iOS in its early stages, it diverged during the development of a formal framework.
Android took a less strict approach in enforcing correct behavior than iOS, as described in detail below. 

\subsubsection{Copy and Paste}
In contrast to iOS, Android does allow clipboard access to background apps~\cite{fahl2013hey}, which can leave credentials vulnerable to theft unless password managers clear the clipboard.

\subsubsection{Accessibility Service}
The first approach that allowed filling passwords into other applications was to leverage the accessibility service provided by Android.
While the purpose of the accessibility service is to help users with disabilities, it has several features that allow it to be used to implement filling passwords (though the developer recommendations do advise against using the accessibility service for non-accessibility purposes).
First, it allows an accessibility app---the password manager in this case---to scan the visual elements being displayed in the current app; this is used by the password manager to identify login forms.
Second, it allows the accessibility app to overlay additional interfaces over the current applications; this is used by the password manager to have the user select which account credentials to fill.
Third, it allows the accessibility app to enter text for the user; this is used by the password manager to actually fill the user's credentials.
One drawback of this approach is it does require the users to give accessibility permissions to the password manager, which is not a straightforward process.
Additionally, research has shown that relying on the accessibility service introduces numerous security vulnerabilities~\cite{fratantonio2017cloak,jang2014a11y,lee2016study,naseri2019accessileaks}.

\subsubsection{Android Autofill Service}
In 2017, Android introduced the autofill service as part of API 26 (Android 8.0---Oreo).\footnote{25\% of Android devices are unable to use the autofill service as they have not, and likely cannot, be upgraded to API 26.}
The autofill service was intended to provide OS-level support for password manager autofill, obviating the need to rely on the accessibility service.
With the autofill service, the OS manages communication between autofill services, such as password managers, and autofill clients, which are the apps that need to be filled.
By default, the autofill service relies on autofill clients to annotate their login interfaces using the \texttt{android:autofillHints} attribute, though the autofill service does have several backup heuristics it can use to identify login forms if the application is not properly annotated.

On Android, the password managers are free to style the autofill credential selection dialog as they see fit.
Figure~\ref{fig:androidautofillui} gives two examples of different UIs on Android.

\subsubsection{OpenYOLO Framework}
Around the same time the autofill service was released, Dashlane (a password manager) and Google worked together to create the OpenYOLO framework.\footnote{\url{https://github.com/openid/OpenYOLO-Android}}
Similar to the autofill service, OpenYOLO was designed to address problems with using the accessibility service to implement autofill.
In OpenYOLO, rather than modifying the Android framework itself (as was done for the autofill service), clients (apps) and servers (password managers) are modified so that the app can receive credentials directly from the password manager.  
The advantage of OpenYOLO over the autofill service is that OpenYOLO is deterministic and allows an app to specify which details it wants to retrieve from a credential provider.
However, because OpenYOLO requires more effort to implement than and was not designed to be interoperable with the autofill service, it has not seen wide adoption.\footnote{\url{https://discussions.agilebits.com/discussion/111985/is-openyolo-dead}}. 
